# Supplementary material for: Graph Neural Network-State Predictive Information Bottleneck (GNN-SPIB) approach for learning molecular thermodynamics and kinetics
Source: arXiv:2409.11843 ancillary file (2024-09-18)
Supplement: Supplementary file 1 [file supplement.pdf]

# Supplementary Information: Graph Neural Network-State Predictive Information Bottleneck (GNN-SPIB) approach for learning molecular thermodynamics and kinetics

Ziyue Zou[1] and Dedi Wang[2,3] and Pratyush Tiwary[1,3,4]

1. Department of Chemistry and Biochemistry, University of Maryland, College Park 20742, USA.
2. Biophysics Program, University of Maryland, College Park 20742, USA.
3. Institute for Physical Science and Technology, University of Maryland, College Park 20742, USA.
4. University of Maryland Institute for Health Computing, Bethesda 20852, USA.

## S1. ENHANCED SAMPLING METHODS

In this section, we provide detailed information about the enhanced sampling methods used in this work along with the parameters adopted.

### A. Well-Tempered Metadynamics

We first test the quality of our learned graph-based SPIB (GNN-SPIB)latent representations by biasing them in well-tempered metadynamics (WTmetaD) [1] and evaluating the accuracy of thermodynamic property estimations. In the next section, we introduce a second evaluation metric. The performance of WTmetaD simulations using these GNN-SPIB variables is assessed by computing the free energy difference between well-studied metastable states of the selected model systems. These values are then benchmarked against those obtained from standard long molecular dynamics simulations and WTmetaD simulations using *a priori* known expert-based CVs.

While standard metadynamics helps the system escape different free energy minima by depositing Gaussian bias potentials onto low-dimensional CVs, it often leads to oscillating rather than converging free energy surfaces [2]. Well-tempered metadynamics (WTmetaD) improves this by scaling the initial bias potential based on the system's history, leading to better free energy convergence. In our work, we limit the biased latent variables, $z$, to two dimensions for efficient sampling, though the models can theoretically learn higher-dimensional representations from atomic Cartesian coordinates which could then be used in other biasing methods which in principle can handle more than two biasing variables. [3]

If our latent representations learned through GNN-SPIB have indeed captured the relevant slow modes, then WTmetaD should estimate thermodynamic properties without hysteresis, i.e., the trajectory should no longer get trapped in metastable states. To evaluate the quality of GNN-SPIB CVs, we first performed WTmetaD simulations to check if GNN-SPIB variables enable robust state-to-state transitions without hysteresis. For all systems, we quantify the hysteresis by visualizing the time series of biasing variable and the corresponding time-dependent free energy surface for state-to-state transitions.

The parameters for WTmetaD simulations for all systems using GNN-SPIB are provided in Tab. S1, where $\omega$ is the initial height of the Gaussian, $\sigma$ is the width of the Gaussian, $\gamma$ is the biasfactor, $T$ is the temperature at which the simulation was carried out, and pace indicates the number of MD integration steps between two bias deposition events. For reference WTmetaD simulation biasing expert-based CVs, we adopted setups from Refs. 4, 5, and 6, for Lennard-Jones 7 cluster, alanine dipeptide, and alanine tetrapeptide, respectively. All metadynamics simulations were performed using PLUMED[7, 8] package with MD engine GROMACS[9–11].The specific versions of these packages are provided in the SI.

### B. Infrequent Metadynamics

We now subject our GNN-SPIB latent variables to an even more demanding test, namely the ability to obtain accurate rare event kinetics through the infrequent metadynamics approach.[12] Although the well-tempered variant of metadynamics (WTmetaD) can converge to accurate free energies[13] , frequent biasing along non-optimal coordinates that overlook relevant slow degrees of freedom corrupts the mechanism and kinetics. To address this, a variant called infrequent metadynamics (imetaD)[12] was developed to provide reliable measurements of transition times (or first passage times) within the metadynamics framework. As the name suggests, imetaD uses a much slower bias deposition rate than conventional WTmetaD, and needs pre-optimized biasing coordinates that approximate the reaction coordinate. If the transition state is assumed to be uncontaminated in a biased simulation, the biased timescale can be properly reweighted by $\alpha(t)t = \int_0^t dt' \exp(\beta V(s,t'))$ for an estimation of the unbiased timescale, where $\beta$ is the inverse temperature, and $V(s,t')$ is the instantaneous bias at $t'$. The characteristic transition time, in short, is estimated by fitting to the empirical cumulative distribution function of a Poisson process.

The reliability of transition time estimation can be assessed using the Kolmogorov–Smirnov (K-S) test as described in Ref. 5. The $p$-value from the K-S test indicates the accuracy of the transition times measured from multiple individual imetaD simulations. A $p$-value greater than 0.05 supports the null hypothesis that the transition times from imetaD simulations and random data points from a Poisson distribution are from the same distribution. To examine the GNN-SPIB latent variables,

TABLE S1: Well-Tempered Metadynamics Parameters.

| System | $\omega(k_BT)$ | $\gamma$ | $\sigma_1$ | $\sigma_2$ | $T(K)$ | pace |
|---|---|---|---|---|---|---|
| LJ7* | 0.5 | 5 | 0.5 | 0.5 | 0.1 | 500 |
| alanine depeptide | 0.5 | 5 | 0.4 | 0.4 | 300 | 500 |
| alanine tetrapeptide | 0.5 | 5 | 0.2 | 0.2 | 350 | 500 |

*LJ7 system is in reduced Lennard-Jones units.

TABLE S2: Infrequent Metadynamics Parameters.

| System | Transition | $\sigma$ | $T(K)$ | pace (steps) | | | First-passage criterion |
|---|---|---|---|---|---|---|---|
| LJ7* | $c_0 \rightarrow c_3$ | 0.1 | 0.1 | 2000 | 10000 | 50000 | $-0.2 < \mu_3^3 < 0.1$ |
| alanine depeptide | $\{C5, C7_{eq}\} \rightarrow C7_{ax}$ | 0.4 | 300 | 2000 | 10000 | 50000 | $0.5 < \phi < 1.5$ |
| alanine tetrapeptide | $s_1 \rightarrow s_7$ | 0.2 | 400 | 200 | 1000 | 5000 | $-0.6\pi < \phi_1 < -0.2\pi$<br>$0.2\pi < \phi_2 < 0.4\pi$<br>$0.5\pi < \phi_3 < 1.5\pi$ |

*LJ7 system is in reduced Lennard-Jones units.

we highlight one slow mode from each model system and perform 100 independent imetaD simulations. The first-passage times (i.e., transition times) are estimated from simulations using (i) long, unbiased MD, (ii) imetaD with expert-designed CVs, and (iii) imetaD with SPIB-GNN CVs. These are collected under the same stop criterion, with various bias deposition frequencies, and fitted to estimate the characteristic transition time. We then compare the robustness of these biasing coordinates, providing qualitative evaluations at the CV level.

The parameters for performing imetaD simulations are provided in Tab. S2. where the $\sigma$ is the width of the Gaussian, $T$ is the temperature at which the simulation was carried out, and pace indicates the number of MD integration steps between two bias deposition events. Bias height $\omega$ and biasfactor $\gamma$ were kept the same as in WTmetaD simulations (see Tab. S1 for their values). For the imetaD parameters, we consulted simulations in Refs. 4,14, and 15 for LJ7, alanine depeptide, and alanine tetrapeptide, respectively.

## S2. PHYSICALLY INSPIRED EXPERT-BASED COLLECTIVE VARIABLES

We start by introducing the known expert-based collective variables used while studying the model systems in this work. All of these CVs are hand-crafted and to some extent require physical knowledge and intuitions *a priori* about the systems of interest.

### A. Lennard-Jones 7 Cluster

In the 2-dimensional Lennard-Jones 7 cluster cluster, the expert-based CVs which are usually considered as reaction coordinates are the second moment of coordination number $c$,

$$\mu_2^2 = \frac{1}{N} \sum_{i=1}^{N} (c_i - \bar{c})^2, \tag{1}$$

and third moment of coordination number,

$$\mu_3^3 = \frac{1}{N} \sum_{i=1}^{N} (c_i - \bar{c})^3, \tag{2}$$

where $\bar{c}$ is the mean of $c$ and $N$ is the number of particles. With these definitions, one may see the key to classifying metastable states in LJ7 system is the fluctuation and distribution of coordination numbers of individual LJ particles, rather than the ensemble average, which the latter could be a typical candidate collective variable to consider in colloidal systems.

### B. Alanine Dipeptide and Alanine Tetrapeptide

Physics-informed CVs in biomolecules like alanine dipeptide and alanine tetrapeptide are representations in higher order (than distances). Explicitly, they are dihedrals $\phi$ and $\psi$. $\phi$ is defined by the angle between displacement vectors C1-N1 and C$\alpha$-C2 projected onto the plane orthogonal to the axis N1-C$\alpha$ and $\psi$ is defined by quadruplet torsion angle of vectors N1-C$\alpha$ and C2-N2 for alanine dipeptide (see main text for atomic labels and graphic definitions). To alanine tetrapeptide, multiple $\phi$ and $\psi$ torsion angles exist and they are all defined in main text.

## S3. GRAPH CONVOLUTION LAYERS

While we provided basic concepts about graph neural nets, here we introduce individual graph convolution layers adopted in the model systems.

### A. LJ7:Equivariant Graph Neural Net

As presented in Fig. 2, the geometric operator consists of three graph convolution layers (denoted as EGCL) developed in Ref. [16]. Here we modified the layer slightly by removing the coordinate input and we directly fed pairwise distances as edge features into these EGCL layers. The message passing function $m$ for node $i$ at layer $l$ is defined by,

$$m_i = \sum_{j \in \mathcal{N}_i \cup \{i\}} \Theta_e(h_i^l \oplus h_j^l \oplus L_{ij}) \tag{3}$$

where $\Theta_e$ is trainable neural net (i.e., MLP), $h$ is the embedding ($h^0 = X$), $L_{ij}$ is the edge feature of edge of nodes $i$ and $j$, and $\oplus$ denotes concatenation. $\Theta$ refers to a trainable neural net with arbitrary subscripts differentiating such operations unless otherwise specified. By introducing node embeddings $h_i$ into the message passing function can be helpful when learning deeper networks. [17] The message is then updated through the function:

$$h_i^{l+1} = h_i^l + \Theta_n(h_i^l \oplus m_i) \tag{4}$$

where $\Theta_n$ is a trainable neural network, and $\mathcal{N}_i$ is the neighborhood of node $i$. Note that a residual connection[18] is added to the update function for better convergence while training. In particular, the hidden EGCL layers in geometric module have 16 neurons and the output embedding is 8-dimensional. This leads to a total of 16-dimensional graph embedding (a concatenation of 8 from mean pooling and 8 from max pooling) to the SPIB module.

### B. Alanine Depeptide:Graph Attention Net

Our second model is composed of two graph attention convolution layers (GAT) from Ref. [19, 20]. Notably, the information from edges are evaluated by a scoring function before updating. The overall process can be expressed as:

$$h_i^{l+1} = \sum_{j \in \mathcal{N}_i} \alpha_{ij} \Theta_t h_j^l \tag{5}$$

where $\alpha_{ij}$ is the attention coefficient normalized a softmax operation over the neighborhood $\mathcal{N}_i$, which indicates the importance of node and edge features of neighboring node $j$ to node $i$ and it is defined as,

$$\alpha_{ij} = \frac{\exp\left(\mathbf{a}^\intercal \mathrm{LeakyReLU}(\Theta_t h_i^l \oplus \Theta_t h_j^l \oplus \Theta_e L_{ij})\right)}{\sum_{j' \in \mathcal{N}_i} \exp\left(\mathbf{a}^\intercal \mathrm{LeakyReLU}(\Theta_t h_i^l \oplus \Theta_t h_{j'}^l \oplus \Theta_e L_{ij'})\right)} \tag{6}$$

where the alignment model $\mathrm{a}^\intercal$ is a trainable feedforward network referred as *self-attention*. [19, 21] The model in this work, we have 16 neurons in the hidden GAT layer and 8 in the output layer. The number of heads is set to be 1. Self-loop is added to the input graph meaning individual nodes are connected to itself and the corresponding edge feature is set to be 0 under Gaussian basis function (see Sec. S4 for details). The negative slope of nonlinearity is 0.2.

### C. Alanine Tetrapeptide:Gaussian Mixture Model

In our last model system, the graph module is constructed with gaussian mixture model convolution layers (GMM) introduced in Ref. [22]. Again, the graph module consists of 2 GMM layers. The embedding at layer $l+1$ is defined as:

$$h_i^{l+1} = \sum_{j \in \mathcal{N}_i} \frac{1}{K} \sum_{k=1}^{K} \mathbf{w}_k(L_{ij}) \cdot \Theta_k h_j^l \tag{7}$$

where $\cdot$ denotes matrix multiplication and $\mathbf{w}$ is parameteric Gaussian kernels with learnable parameters whose expression is,

$$\mathbf{w}_k(L) = (-\frac{1}{2}(L - \mu_k)^\intercal \Sigma_k^{-1}(L - \mu_k)) \tag{8}$$

where $\mu_k$ and $\Sigma_k^{-1}$ are learnable mean vector and covariance matrix of Gaussian kernels, respectively, and $k$ is the total number of kernel functions. Given geometric data in this work only contains pair-wise distances as edge feature, the value of $k$ in this architecture is the dimensionality of edge feature via message passing. The hidden GMM layer has 64 channels and the output GMM layer has 16 channels. The kernel size $k$ is 20. In addition, we apply a jumping knowledge skip connection [23] to the hidden GMM layer, which means the hidden embedding is concatenated to the output embedding before global pooling layers. This operation in general is beneficial while training deeper neural nets but we also find this improves the performance to our model.

## S4. GEOMETRIC DATA PREPARATION AND SIMULATION SETUPS

The pipeline involves graph module and SPIB module, which suggests the input data should not only be continuous at least in a time interval, but in its geometric representation. In the following section, we show how we construct our training data from MD trajectories.

### A. Lennard-Jones 7 cluster

To LJ7 system, we performed the simulation at a temperature $k_B T = 0.2\epsilon$ using Langevin thermostat for $1 \times 10^7$ steps. The simulation was performed at a higher temperature for efficient sampling in the configuration space. The coupling time of the thermostat is 0.1 $\sqrt{\epsilon/m\sigma^2}$. The equation of motion is integrated with a time step 0.005 $\sqrt{\epsilon/m\sigma^2}$. The simulation was performed in PLUMED-2.8.1 with PYTORCH module. The 2-d coordinates of all particles were saved every 10 steps, leading to $1 \times 10^6$ snapshots in total. We then computed all pair-wise distances in each frame and constructed their geometric representations. All graphs were set to be fully-connected.

Besides graph representations to the simulation cell, SPIB model require a psudo state label for individual time frame, here we assigned 8 initial labels using K-means clustering algorithm [24] in $\{\mu_2^2, \mu_3^3\}$ space.

### B. Alanine Dipeptide

The alaine dipeptide in vacuum simulation for generating training data was performed at 450 $K$ using stochastic velocity rescaling thermostat. The force field was selected to be AMBER99SB and the integration time step was 2 $fs$. The simulation was performed in GROMACS-2019.6 package and the atomic coordinates were saved every 50 steps for 200 $ns$. 2 $\times 10^6$ configurations were converted into their graph representations. Complete (fully-connected) graphs are construct when training and biasing the machine learning models.

As introduced in the main text, conformational changes in alanine dipeptide can easily be characterized by high-order torsion angles but they are non-trivial when using pure distances. Following the definition of dihedral, the two intersecting planes in computation of a dihedral angle rely on the displacement vectors between the four atoms (points) in atomic simulations. However, this piece of information is lost in graph construction to enforce the invariance to translations and rotations in the embeddings in GNNs. Under this consideration, we defined our neighboring metric to a large radius cutoff, $r_{cut} = 1.0\ nm$, as mentioned earlier and this again let the graph objects be fully connected. The 8 initial state labels were generated with k-means clustering in $\{\phi, \psi\}$ space.

### C. Alanine Tetrapeptide

Alaine tetrapeptide in vacuum simulations were performed at 400 $K$ for 1.0 $\mu s$ with a time step of 2 $fs$ and AMBER99SB forcefield. Atom coordinates were saved every 500 steps. The thermostat was selected to be stochastic velocity rescaling thermostat with a relaxation time of 0.1 $ps$.

Similar to alanine depeptide, the constructed graphs in alanine tetrapeptide should remain fully-connected, which leads to high dimensional input feature, $\mathrm{C}(20, 2)$ = 190-d, which original SPIB model may have difficulty handling. However, we did realize an advantage of GNNs or data in their geometric form is the focus of neighboring nodes and making a fully-connected graph does not make GNN any special to standard convolutional neural networks (CNNs) when permutation invariant property is not strictly needed (like in alanine depeptide and alanine tetrapeptide). However, it seems critical to take more features into account if only type-0 representations are involved. Therefore, We will leave this objective of constructing smaller graphs using narrower radius cutoff for future researches. The 24 initial state labels to alanine tetrapeptide were generated with k-means clustering in $\{\phi_1, \phi_2, \phi_3\}$ space.

## S5. MODEL TRAINING AND ANALYSIS

Before presenting all parametering while training our model, we briefly introduce some of our parameters. They are mainly from the original SPIB method, and detailed description can be found in the original work. [25] Since SPIB model is optimizing predictions to the future, a lagtime parameter, $\Delta t$, which control how far in time the model should look into is defined and this timescale should smaller (or faster) than the fastest transitions of interest. A $\beta$ term is assigned to the KL divergence term and it is used to balance the two losses in the objective function. To optimization, three parameters, tolerance to loss change $\mathcal{L}_{tol}$, patience $P$ and number of refinements $N_{ref}$ need to be specified, and they define when the optimization should be terminated and the training is converged. Smaller $\mathcal{L}_{tol}$ leads to more metastable states, and longer training/convergence time. Larger patience or number of refinements, results in better-defined state boundary.

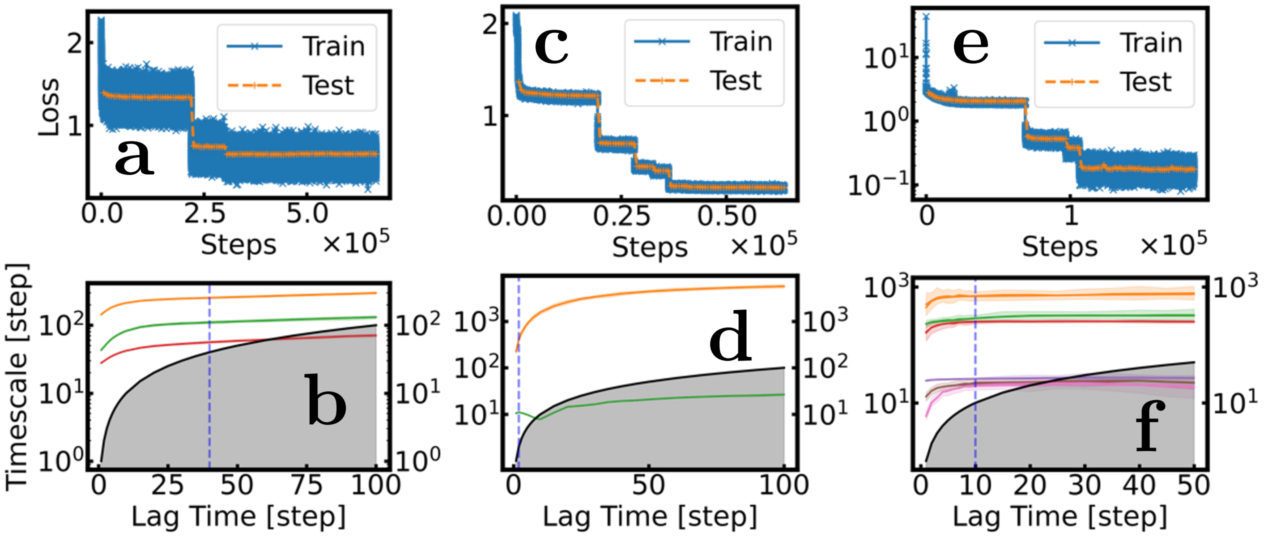


**FIG. S1:** Analyses to trained models of LJ7 (left panel; a-b), alanine depeptide (middle panel; c-d), and alanine tetrapeptide (right panel; e-f) systems. The remaining number of states vs. the number of refinements plots are shown on the first row (subplots a, e, and i). The second row (b, f, and j) is the change in state population vs. the number of steps plot. The third row (c, g, and k) traces the loss change. Overall, all these three types of plots were indicators of converged trains. On the last row (d, h, and l), the implied timescales plots for our trained model. The dashed lines correspond to the lag time defined when training models in this work.

### A. Lennard-Jones 7 cluster

The time delay $\Delta t$ was set to be 40 $\sqrt{\epsilon/m\sigma^2}$. The GCL layers in the model had 8 channels, and both the encoder and the decoder had 16 channels. $\mathcal{L}_{tol}$, $P$, and $N_{ref}$ were set to be $5 \times 10^{-4}$, 3, and 12, respectively. The ratio of train and test datasets is 80 : 20. The model was optimized with Adam optimizer[26] with a learning rate of $1 \times 10^{-3}$. The value of $\beta$ was set to be $1 \times 10^{-2}$. The batch size of the graph objects was 128. To graphs, batching results in a much larger graph in which nodes from different graphs are not connected.

In FigS1 left panel, we summarize the result of training, in subplot a, the loss gradually drops until plateau within $2.5 \times 10^5$ epochs. In FigS1d), we plot the implied timescales with our trained model. The three slowest transitions were plotted and the selected time delay was less than these transition times. In particular, the corresponding slow modes can be identified by their eigenvectors. Referring to Fig. S2a), the first eigenvector corresponds to the stationary distribution. The second eigenvector is the transition between $c_0$ and $c_3$. The third eigenvector is the transition between $c_1$ and $c_3$ and the last eigenvector is the transition between $c_2$ to $c_3$ and $c_1$.

### B. Alanine Dipeptide

The lag time $\Delta t$ was set to be 0.2 $ps$. We had 8 channels for the GAT layers and 16 neurons for all other linear layers. All GAT layers had 1 head and the slope of the leaky ReLU was set to be 0.1. $\mathcal{L}_{tol}$, $P$, and $N_{ref}$ were set to be $5 \times 10^{-4}$, 3, and 12, respectively. The value of batch size was 2560 and hyperparameter $\beta$ was set to be $1 \times 10^{-3}$. When training on the model, Adam optimizer was used with a learning rate of $1 \times 10^{-3}$. 80% of the input dataset was used for training, and the remaining 20% was the test dataset.

As shown in Fig. S1 middle panel subplot c), loss converges after around $3.5 \times 10^4$ training steps. The implied timescales plot (subplot d) shows the timescale of two transitions. As suggested by Fig. S2b, the slowest transition (i.e., the second eigenvector) is between C7$_{ax}$ and {C5,C7$_{eq}$}. The second transition (the $3^{rd}$ eigenvector) is between C5 and C7$_{eq}$.

### C. Alanine Tetrapeptide

The lag time $\Delta t$ for alanine tetrapeptide was set to be 10 $ps$. We had 16 channels for the GMM layers with 20 kernels. The encoder had 64 hidden channels and the decoder had 16 channels. $\mathcal{L}_{tol}$, $P$, and $N_{ref}$ were set to be $1 \times 10^{-3}$, 3, and 12, respectively. The dataset was batched to a batch size of 512 and $\beta$ was set to be $1 \times 10^{-2}$. The model was trained using the Adam optimizer with a learning rate of $1 \times 10^{-3}$. The dataset was split into 80% vs. 20% for train and test sets. The number

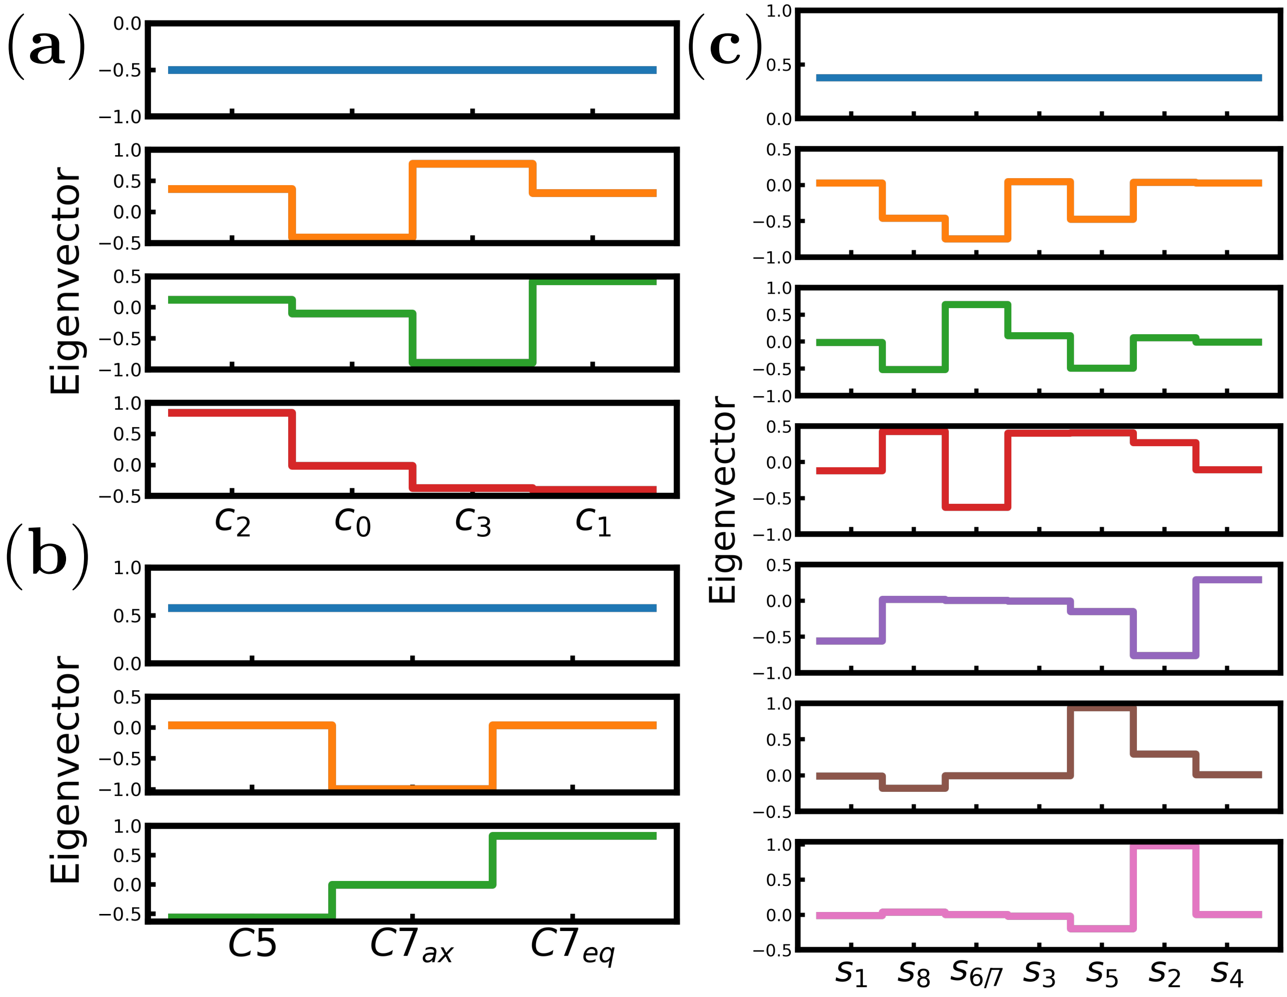


**FIG. S2:** Eigenvectors of (a) LJ7, (b) alanine depeptide, and (c) alanine tetrapeptide. The first eigenvector of each system corresponds to the stationary probability distribution, and the rest of the eigenvectors present the slow transitions with the trained models in ascending order, which means the second eigenvector is the transition with the longest timescale to the system.

of states, as suggested by Fig. S1e), loss is converged after $1 \times 10^5$ steps. In subplot f, the 6 transition timescales are identified and they are relatively slow to the selected time lag, $\Delta t$. The slowest transition (see Fig. S2c) second eigenvector in orange) is the transition between $S_{6/7}$ and $\{S_1, S_2, S_3, S_4\}$. The second slowest transition corresponds to the interplay between $S_{6/7}$ and $\{S_8, S_5\}$. After this, the rest slow transitions are $S_{6/7} \leftrightarrow \{S_3, S_5, S_8\}$, $S_2 \leftrightarrow S_4$, $S_5 \leftrightarrow S_8$, and $S_5 \leftrightarrow S_2$.

## S6. SUMMARY FOR THE PERFORMED WELL-TEMPERED METADYNAMICS AND INFREQUENT METADYNAMCIS SIMULATIONS

In this section, we provided numerical values to the box plots of free energy differences using WTmetaD's and scatter plots of the kinetic measurements using imetaD's. Definition of these terms can be found in main text with detailed explanation.

## S7. ATTENTION COEFFICIENTS IN ALANINE DEPEPTIDE SYSTEM

In graph attention networks, attention coefficients are computed during message passing. These coefficients indicate the importance of individual edges within individual graphs (see Sec. S3 B). We therefore post-process one production run by computing the coefficient matrices every time frame. The Boltzmann-weighted time-averaged attention coefficient matrix of the two GAT layers were plotted in Fig. S3. It is clear that, the two layers capture different physical information — the first

# TABLE S3: Well-tempered Metadynamics Results

| System | Unit | Transition | MD | WTmetaD (expert-based) | WTmetad (GNN-SPIB) |
|---|---|---|---|---|---|
| LJ7 | $\epsilon$ | $c_0 \rightarrow c_1$ | 0.644 ± 0.013 | 0.642 ± 0.007 | 0.631 ± 0.010 |
| | | $c_0 \rightarrow c_2$ | 0.643 ± 0.013 | 0.641 ± 0.008 | 0.631 ± 0.010 |
| | | $c_0 \rightarrow c_3$ | 0.795 ± 0.031 | 0.765 ± 0.023 | 0.759 ± 0.016 |
| alanine depeptide | $kJ/mol$ | $C7_{eq} \rightarrow C5$ | -0.040 ± 0.002 | -0.023 ± 0.049 | -0.083 ± 0.064 |
| | | $C7_{eq} \rightarrow C7_{ax}$ | 7.59 ± 0.92 | 7.60 ± 0.13 | 7.48 ± 0.21 |
| alanine tetrapeptide | $kJ/mol$ | $s_1 \rightarrow s_2$ | 14.19 ± 0.75 | 14.01 ± 0.42 | 14.06 ± 0.94 |
| | | $s_1 \rightarrow s_3$ | 1.57 ± 0.33 | 1.42 ± 0.22 | 1.50 ± 0.35 |
| | | $s_1 \rightarrow s_4$ | -1.01 ± 0.07 | -0.97 ± 0.05 | -0.79 ± 0.11 |
| | | $s_1 \rightarrow s_5$ | 13.53 ± 1.34 | 13.46 ± 0.68 | 13.25 ± 0.48 |
| | | $s_1 \rightarrow s_6$ | 21.13 ± 2.74 | 20.90 ± 1.37 | 21.47 ± 0.98 |
| | | $s_1 \rightarrow s_7$ | 12.88 ± 3.41 | 11.99 ± 0.90 | 12.38 ± 0.55 |
| | | $s_1 \rightarrow s_8$ | 9.54 ± 1.10 | 9.36 ± 0.53 | 9.30 ± 0.44 |

# TABLE S4: Infrequent Metadynamics Results

| System | Unit | Transition | Pace | Biasing variable(s) | Characteristic transition time | 95% Confidence Interval | $p$-value |
|---|---|---|---|---|---|---|---|
| LJ7 | $\sqrt{\epsilon/(m*\sigma^2)}$ | $c_0 \rightarrow c_3$ | 2000 | $\mu_2^2$ | 662144 | [848945, 1598062] | 0.0067 |
| | | | | $\mu_3^3$ | 46700 | [39969, 58738] | 0.5278 |
| | | | | $z_1$ | 48007 | [46669,81944] | 0.4579 |
| | | | | $z_2$ | 69850 | [59995,93118] | 0.9185 |
| | | | 10000 | $\mu_2^2$ | 288189 | [355139, 621122] | 0.0382 |
| | | | | $\mu_3^3$ | 47955 | [39000, 55565] | 0.7389 |
| | | | | $z_1$ | 53829 | [46282,73303] | 0.9845 |
| | | | | $z_2$ | 64504 | [52986,77703] | 0.9492 |
| | | | 50000 | $\mu_2^2$ | 190080 | [167219, 262661] | 0.9354 |
| | | | | $\mu_3^3$ | 59990 | [384000, 55565] | 0.8549 |
| | | | | $z_1$ | 66216 | [55114,80000] | 0.9633 |
| | | | | $z_2$ | 50246 | [42775,63531] | 0.9088 |
| | | | - | - | 60630 | [46945, 66598] | 0.4637 |
| alanine depeptide | $ns$ | $C7_{eq} \rightarrow C7_{ax}$ | 2000 | $\phi$ | 4164 | [4091, 7390] | 0.4272 |
| | | | | $\psi$ | 70295 | [3551058, 14685901] | 0.0000 |
| | | | | $z_1, z_2$ | 4839 | [4821,7862] | 0.3414 |
| | | | 10000 | $\phi$ | 3942 | [3347, 4964] | 0.7214 |
| | | | | $\psi$ | 24031 | [92489, 546832] | 0.0001 |
| | | | | $z_1, z_2$ | 4424 | [3662, 5384] | 0.7488 |
| | | | 50000 | $\phi$ | 1826 | [3347, 4475] | 0.9006 |
| | | | | $\psi$ | 11555 | [12445, 21610] | 0.0956 |
| | | | | $z_1, z_2$ | 4226 | [3798, 6030] | 0.8285 |
| | | | - | - | 3340 | [2857, 4259] | 0.8849 |
| alanine tetrapeptide | $ns$ | $s_1 \rightarrow s_7$ | 200 | $\phi_1, \phi_2, \phi_3$ | 288 | [244, 377] | 0.9369 |
| | | | | $\psi_1, \psi_2, \psi_3$ | 3553 | [34790, 163661] | 0.0000 |
| | | | | $z_1, z_2$ | 643 | [615,1028] | 0.8605 |
| | | | 1000 | $\phi_1, \phi_2, \phi_3$ | 398 | [340, 509] | 0.7799 |
| | | | | $\psi_1, \psi_2, \psi_3$ | 3635 | [7797, 20400] | 0.0025 |
| | | | | $z_1, z_2$ | 460 | [378, 618] | 0.7879 |
| | | | 5000 | $\phi_1, \phi_2, \phi_3$ | 412 | [311, 471] | 0.6821 |
| | | | | $\psi_1, \psi_2, \psi_3$ | 1293 | [2268, 4881] | 0.0004 |
| | | | | $z_1, z_2$ | 394 | [343, 527] | 0.6937 |
| | | | - | - | 489 | [409, 612] | 0.9728 |

"–" suggests the MD simulations were conducted instead of imetaD simulations.

layer (subplot a) emphasizes on the nodes with are far away from each other, while the second layer (subplot b) focuses on the local orientation of neighboring nodes.

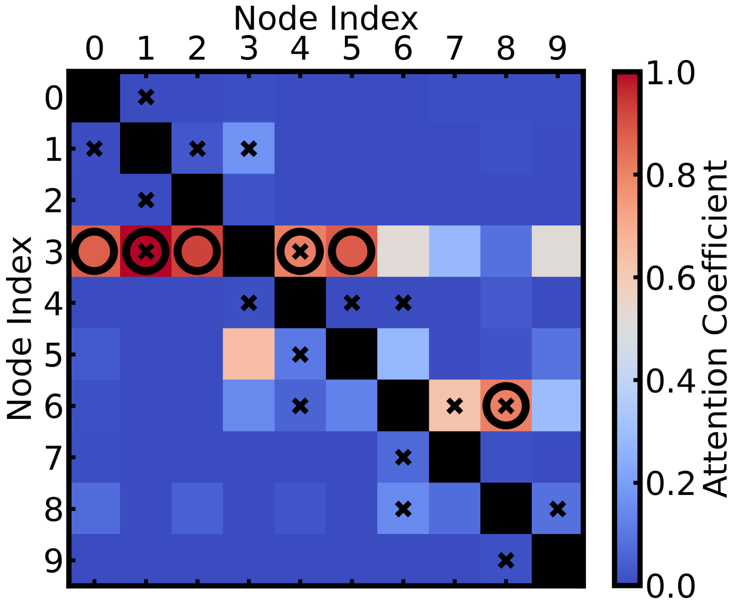


**FIG. S3:** Attention coefficients for the first (a) and the second (b) GAT layer from one production run. The value of coefficient was computed from by weighted average from the entire simulation.

## SUPPLEMENTARY REFERENCES


[1] Omar Valsson, Pratyush Tiwary, and Michele Parrinello. Enhancing important fluctuations: Rare events and metadynamics from a conceptual viewpoint. Annual review of physical chemistry, 67:159–184, 2016.

[2] Federico Giberti, Matteo Salvalaglio, Marco Mazzotti, and Michele Parrinello. Insight into the nucleation of urea crystals from the melt. Chemical Engineering Science, 121:51–59, 2015.

[3] Lula Rosso and Mark E. Tuckerman. An adiabatic molecular dynamics method for the calculation of free energy profiles. Molecular Simulation, 28(1-2):91–112, 2002.

[4] Gareth A. Tribello, Michele Ceriotti, and Michele Parrinello. A self-learning algorithm for biased molecular dynamics. Proceedings of the National Academy of Sciences, 107(41):17509–17514, 2010.

[5] Matteo Salvalaglio, Pratyush Tiwary, and Michele Parrinello. Assessing the reliability of the dynamics reconstructed from metadynamics. J. Chem. Theor. Comp., 10(4):1420–1425, 2014.

[6] Jakub Rydzewski and Omar Valsson. Multiscale reweighted stochastic embedding (mrse): Deep learning of collective variables for enhanced sampling. arXiv preprint arXiv:2007.06377, 2020.

[7] Gareth A. Tribello, Massimiliano Bonomi, Davide Branduardi, Carlo Camilloni, and Giovanni Bussi. Plumed 2: New feathers for an old bird. Comp. Phys. Comm., 185(2):604–613, 2014.

[8] Massimiliano Bonomi, Giovanni Bussi, and Carlo Camilloni Camilloni. Promoting transparency and reproducibility in enhanced molecular simulations. Nat. Methods., 16:670–673, 2019.

[9] Herman JC Berendsen, David van der Spoel, and Rudi van Drunen. Gromacs: a message-passing parallel molecular dynamics implementation. Comp. Phys. Commun., 91(1-3):43–56, 1995.

[10] Abraham Mark James Szilárd, Páll, Carsten Kutzner, Berk Hess, and Erik Lindahl. Tackling exascale software challenges in molecular dynamics simulations with gromacs. Solving Software Challenges for Exascale, 8759:3–27, 2015.

[11] Mark James Abraham, Teemu Murtola, Roland Schulz, Szilard Pall, Jeremy C Smith, Berk Hess, and Erik Lindahl. Gromacs: High performance molecular simulations through multi-level parallelism from laptops to supercomputers. SoftwareX, 1:19–25, 2015.

[12] Pratyush Tiwary and Michele Parrinello. From metadynamics to dynamics. Physical review letters, 111(23):230602, 2013.

[13] James F. Dama, Michele Parrinello, and Gregory A. Voth. Well-tempered metadynamics converges asymptotically. Phys. Rev. Lett., 112:240602, Jun 2014.

[14] Ofir Blumer, Shlomi Reuveni, and Barak Hirshberg. Short-time infrequent metadynamics for improved kinetics inference. Journal of Chemical Theory and Computation, 20(9):3484–3491, 2024. PMID: 38668722.

[15] Ofir Blumer, Shlomi Reuveni, and Barak Hirshberg. Combining stochastic resetting with metadynamics to speed-up molecular dynamics simulations. Nature Communications, 15(1):240, Jan 2024.

[16] Victor Garcia Satorras, Emiel Hoogeboom, and Max Welling. E(n) equivariant graph neural networks. CoRR, abs/2102.09844, 2021.

[17] Tian Xie and Jeffrey C Grossman. Crystal graph convolutional neural networks for an accurate and interpretable prediction of material properties. Physical review letters, 120(14):145301, 2018.

[18] Kaiming He, Xiangyu Zhang, Shaoqing Ren, and Jian Sun. Deep residual learning for image recognition. In 2016 IEEE Conference on Computer Vision and Pattern Recognition (CVPR), pages 770–778, 2016.

[19] Petar Veličković, Guillem Cucurull, Arantxa Casanova, Adriana Romero, Pietro Liò, and Yoshua Bengio. Graph attention networks, 2018.

[20] Shaked Brody, Uri Alon, and Eran Yahav. How attentive are graph attention networks?, 2022.

[21] Dzmitry Bahdanau, Kyunghyun Cho, and Yoshua Bengio. Neural machine translation by jointly learning to align and translate, 2016.

[22] Federico Monti, Davide Boscaini, Jonathan Masci, Emanuele Rodolà, Jan Svoboda, and Michael M. Bronstein. Geometric deep learning on graphs and manifolds using mixture model cnns, 2016.

[23] Keyulu Xu, Chengtao Li, Yonglong Tian, Tomohiro Sonobe, Ken ichi Kawarabayashi, and Stefanie Jegelka. Representation learning on graphs with jumping knowledge networks, 2018.

[24] S. Lloyd. Least squares quantization in pcm. IEEE Transactions on Information Theory, 28(2):129–137, 1982.

[25] Dedi Wang and Pratyush Tiwary. State predictive information bottleneck. The Journal of Chemical Physics, 154(13):134111, 2021.

[26] Diederik P. Kingma and Max Welling. Auto-encoding variational bayes. 2nd International Conference on Learning Representations, ICLR 2014 - Conference Track Proceedings, (Ml):1–14, 2014.
